# Supplementary material for: Pre-training Co-evolutionary Protein Representation via A Pairwise Masked Language Model
Source: arXiv:2110.15527 source file (2021-10-29)
Supplement: Supplementary file 1 [file appendix.tex]

\section{Appendix}

TODO
